# Supplementary material for: Low-Rank Tucker Approximation of a Tensor From Streaming Data
Source: arXiv:1904.10951 source file (2021-04-30)
Supplement: Supplementary file 1 [file compression_sketchy.tex]

\section{Probabilistic Analysis of the Compression Error}

\begin{lem}
\label{lemma: compression_error}
For any natural numbers $\rho_n$, $1\le \rho_n<k_n-1$,
\begin{equation}
\mathbb{E}  \|\tilde{\T{X}} - \T{X}\|_F^2 \le \sum_{n=1}^N \left(1+\frac{\rho_n}{k-\rho_n-1}\right)(\tau^{(n)}_{\rho_n})^2,\nonumber
\end{equation}
where $\tilde{\T{X}}$ is the two pass approximation defined in \eqref{eq:x_tilde}.
\begin{proof}
This proof extends the result for matrix sketching stated in \cite{halko2011finding} to the tensor case.
To construct a similar bound, we first decompose the square norm of the compression error
into the sum of square norms of the differences $\T{Y}_{n-1} - \T{Y}_{n}$ in \eqref{eq: y_diff},
and then bound each term individually in \eqref{eq: y_diff_bound}.
Again, we will show that the inner products between these differences are always zero.

Following the definition of $\T{Y}_n$ in \cref{eq:definition_Y_n},
\begin{equation}\label{eq: y_diff}
\begin{aligned}
& \|\T{X}-\tilde{\T{X}}\|_F^2 = \|\T{Y}_0 - \T{Y}_N\|_F^2= \left\|\sum_{n=0}^{N-1} (\T{Y}_n - \T{Y}_{n+1})\right\|_F^2.
\end{aligned}
\end{equation}
For any $0 \leq m \leq N-1$,
\begin{equation}
\T{Y}_m-\T{Y}_{m+1} = \T{Y}_{m} \times_{(m+1)} (\mathbf{I} - \mathbf{Q}_{m+1}\mathbf{Q}^\top_{m+1}). \nonumber
\end{equation}
and for any $0\le m< n < N$, define $\T{A}^{(m,n)}$ using the equation
$\T{Y}_n - \T{Y}_{n+1} =$
\begin{multline}
\underbrace{\left[\T{X}\times_1 \mathbf{Q}_{1}\mathbf{Q}^\top_{1} \times_2 \cdots \times_{m} \mathbf{Q}_{m}\mathbf{Q}^\top_{m}\times_{(m+2)} \cdots  \times_{n} \mathbf{Q}_{n}\mathbf{Q}^\top_{n}\times_{(n+1)}(\mathbf{I}-\mathbf{Q}_{(n+1)}\mathbf{Q}^\top_{(n+1)})\right]}_{\T{A}}\\
	\times_{(m+1)} \mathbf{Q}_{m+1}\mathbf{Q}^\top_{m+1}.\nonumber
\end{multline}
The second part of \cref{lemma:projection_tensors} shows
\begin{equation}\label{eq:inner_prod1}
\langle\T{Y}_m-\T{Y}_{m+1},  \T{Y}_n - \T{Y}_{n+1}\rangle = \langle\T{Y}_{m} \times_{(m+1)} (\mathbf{I} - \mathbf{Q}_{m+1}\mathbf{Q}^\top_{m+1}), \T{A}^{(m,n)} \times_{m+1} \mathbf{Q}_{m+1}\mathbf{Q}^\top_{m+1} \rangle = 0.\nonumber
\end{equation}
Hence we can decompose the error in the two pass approximation as
\begin{equation}
\label{eq:comression_decomposition}
\begin{aligned}
& \|\T{X}-\tilde{\T{X}}\|_F^2 =  \sum_{n=0}^{N-1} \| (\T{Y}_n - \T{Y}_{n+1})\|_F^2
\end{aligned}
\end{equation}
by the Pythagorean theorem.
Now we bound $\|\T{Y}_n - \T{Y}_{n+1}\|_F^2$ for each $n$:
\begin{equation} \label{eq: y_diff_bound}
\begin{aligned}
\|\T{Y}_n - \T{Y}_{n+1}\|_F^2 &= \|\T{X}\times_{(n+1)} (\mathbf{I} - \mathbf{Q}_{n+1}\mathbf{Q}_{n+1}^\top)\times_{1} \mathbf{Q}_{1}\mathbf{Q}_{1}^\top\dots \times_n \mathbf{Q}_{n}\mathbf{Q}_{n}^\top\|_F^2 \\
&\le \|\T{X}\times_{(n+1)} (\mathbf{I} - \mathbf{Q}_{n+1}\mathbf{Q}_{n+1}^\top)\|_F^2 \\
&= \| (\mathbf{I} - \mathbf{Q}_{n+1}\mathbf{Q}_{n+1}^\top)\mathbf{X}^{(n)}\|_F^2,
\end{aligned}
\end{equation}
where the second line follows from the fact that the projection is contractive,
together with second part of \cref{lemma:projection_tensors}.
Apply \cref{lemma:sketchy_column_space_err} to the last line of the inequality above to show
\begin{equation}
\mathbb{E} \|\T{Y}_n - \T{Y}_{n+1}\|_F^2 \le \left(1+\frac{\rho_n}{k_n-\rho_n-1}\right)(\tau^{(n+1)}_{\rho_n})^2.\nonumber
\end{equation}
Sum the bound for each term in  \eqref{eq:comression_decomposition} to finish the proof.
\end{proof}
\end{lem}
