# Supplementary material for: Low-Rank Tucker Approximation of a Tensor From Streaming Data
Source: arXiv:1904.10951 source file (2021-04-30)
Supplement: Supplementary file 2 [file proof_for_main_results.tex]

\section{Proof of Main Results}
\label{appendix:proof-main-result}

\subsection{Error bound for the two pass approximation \cref{alg:two_pass_low_rank_appro}}
\begin{proof}[Proof of \cref{thm:low_rank_err_two_pass}]
Suppose $\T{\hat{X}}_2$ is the low-rank approximation from \cref{alg:two_pass_low_rank_appro}.
Use the definition of the mode-$n$ product to see
\begin{equation*}
\begin{aligned}
\T{\hat{X}}_2 &=  \left[\T{X}\times_1 \mathbf{Q}_1^\top \times_2 \cdots \times_N \mathbf{Q}_N^\top\right] \times_1 \mathbf{Q}_1\times_1 \cdots\times_N \mathbf{Q}_N\\
&= \T{X}\times_1 \mathbf{Q}_1\mathbf{Q}_1^\top \times_2 \cdots \times_N \mathbf{Q}_N\mathbf{Q}_N^\top.
\end{aligned}
\end{equation*}
Although it seems that we sequentially project tensor $\T{X}$ to column space spanned with $\mathbf{Q}_n$, but since mode product is exchangeable, in fact $\hat{\T{X}}_2$ is the projection to space $\{ \T{X} : \T{X}^{(n)}
\in \range(\mathbf{Q}_n) \}$.  This is a generalization of projection matrix where \cite{de2008tensor} has a very detailed  explanation and it is referred as multi-linear orthogonal projection.  Following exact techniques in Theorem 5.1 in \cite{vannieuwenhoven2012new} by sequentially applying Pythagorean theory we can show that
\begin{equation}
\|\hat{\T{X}}_2 - \T{X}\|_F^2 \le \sum_{n=1}^N  \left \| (\mathbf{I} - \mathbf{Q}_n\mathbf{Q}_n^\top) \mathbf{X}^{(n)} \right\|_F^2 .
\end{equation}
Then taking expectation on $\mathbf{Q}_n$, and applying Lemma \ref{lemma:sketchy_column_space_err} we complete the proof.

\end{proof}

\subsection{Error bound for the one pass approximation \cref{alg:one_pass_low_rank_appro}}
\begin{proof}[Proof of \cref{thm:low_rank_err}]
We show the approximation error can be decomposed as
the error due to the factor matrix approximations
and the error due to the core approximation.
\mnote{Instate this notation in the main body of the paper.}
Let $\T{\hat{X}}_1$ be the one pass approximation from \cref{alg:one_pass_low_rank_appro}, and let
\begin{equation}
\T{\hat{X}}_2 = \T{X}\times_1 \mathbf{Q}_1\mathbf{Q}_1^\top \times_2 \cdots \times_N \mathbf{Q}_N\mathbf{Q}_N^\top,
\end{equation}
be the two pass approximation from \cref{alg:two_pass_low_rank_appro}.
The difference in one-pass and two-pass approximation is in the
core:
\begin{equation}
\begin{aligned}
\T{\hat{X}}_1-\hat{\T{X}}_2= (\T{W}-\T{X}\times_1 \mathbf{Q}_1^\top \times_2 \cdots \times_N \mathbf{Q}_n^\top)  \times_1 \mathbf{Q}_1 \dots \times_N \mathbf{Q}_N. \nonumber
\end{aligned}
\end{equation}
Thus $\T{\hat{X}}_1-\hat{\T{X}}_2$ is in the space defined above:  $\{ \T{X} : \T{X}^{(n)}
\in \range(\mathbf{Q}_n) \}$ while $\hat{\T{X}}_2 - \T{X}$ is orthogonal to that space.  Therefore,

\begin{equation}
\label{eq:inner_zero}
\langle \hat{\T{X}}_1 - \hat{\T{X}}_2, \hat{\T{X}}_2 - \T{X} \rangle = 0.
\end{equation}

Now we use the (expectation of) the Pythagorean theorem
to bound the expected error of the one pass approximation (\cref{eq:error_decom}):
\begin{equation}
%\label{eq:error_decom}
 \mathbb{E}\| \hat{\T{X}}_1- \T{X} \|_F^2 = \mathbb{E}\| \hat{\T{X}}_1 - \hat{\T{X}}_2\|_F^2 + \mathbb{E} \|\hat{\T{X}}_2 - \T{X} \|_F^2.
\end{equation}

Consider the first term which is due to core approximation. Based in the definition of $\hat{\T{X}}_1$ and $\tilde{\T{X}}_2$ we can see that
\begin{align*}
\|\hat{\T{X}}_1 - \hat{\T{X}}_2\|^2_F &=
\|(\T{W}_1 - \T{X}\times_1 \mathbf{Q}_1^\top \cdots \times_N \mathbf{Q}^\top_N)\times_1 \mathbf{Q}_1\cdots \times_N \mathbf{Q}_N \|^2_F\\
& = \|(\T{W}_1- \T{X}\times_1 \mathbf{Q}_1^\top \cdots \times_N \mathbf{Q}^\top_N)\|_F^2,
\end{align*}
where we use the invariance of the Frobenius norm under orthonormal transformations to get the second line.
Now using \cref{lemma:err_core_sketch} to bound for the error due to the core approximation as
%(the first term in \eqref{eq:error_decom}) as
\begin{equation}
\mathbb{E} \|\hat{\T{X}}_1- \hat{\T{X}}_2\|^2_F \le \Delta \left[ \sum_{n=1}^N \left(1+\frac{\rho_n}{k_n-\rho_n-1}\right)(\tau^{(n)}_{\rho_n})^2\right].\nonumber
\end{equation}

Finally, as shown in proof for  \cref{thm:low_rank_err_two_pass} to
bound the error due to the factor matrix approximations
(the second term in \eqref{eq:error_decom}) as
\begin{equation}
\mathbb{E}\|\hat{\T{X}}_2 - \T{X} \|_F^2 \le \left[ \sum_{n=1}^N \left(1+\frac{\rho_n}{k_n-\rho_n-1}\right)(\tau^{(n)}_{\rho_n})^2\right].\nonumber
\end{equation}
Summing these two bounds finishes the proof.
\end{proof}

\subsection{Error bound for the fixed rank approximation \cref{alg:fix_rank_appro}}

\begin{proof}[Proof of \cref{thm:fix_rank_err}]
Our argument for first part follows the proof of \cite[Proposition 6.1]{tropp2017practical}:
\begin{equation}
\begin{aligned}
&\|\T{X} - \llbracket \hat{\T{X}} \rrbracket_\mathbf{r}\|_F\\
&  \le \|\T{X} -  \hat{\T{X}}\|_F+\|\hat{\T{X}} -  \llbracket\hat{\T{X}}\rrbracket_\mathbf{r}\|_F\\
&\le \|\T{X} -  \hat{\T{X}}\|_F+\|\hat{\T{X}} -  \llbracket \T{X}\rrbracket_\mathbf{r}\|_F \\
& \le \|\T{X} -  \hat{\T{X}}\|_F+\|\hat{\T{X}} - \T{X}  + \T{X} - \llbracket \T{X}\rrbracket_\mathbf{r}\|_F \\
&\le 2\|\T{X} - \hat{\T{X}} \|_F + \|\T{X} -  \llbracket \T{X} \rrbracket_\mathbf{r}\|_F.\nonumber
\end{aligned}
\end{equation}
The first and the third line are the triangle inequality,
and the second line follows from the definition of the best rank-$r$ approximation.
Take the expectation of $\|\T{X} - \hat{\T{X}} \|_F$ and
use Jensen's inequality $\mathbb{E}\|\T{X} - \hat{\T{X}} \|_F \le \sqrt{\mathbb{E} \|\T{X} - \hat{\T{X}} \|_F^2}$
to finish the proof. \par
Now we go to the proof for second part,
\begin{equation}
\begin{aligned}
& \|\T{X} - \llbracket \hat{\T{X}}\rrbracket_{\mathbf{A}-\mathbf{r}} \|_F  \\
& \le  \|\T{X} - \T{\hat{X}}\|_F + \|\T{\hat{X}} - \llbracket \hat{\T{X}}\rrbracket_{\mathbf{A}-\mathbf{r}} \|_F & \\
& \le F_2(N)\|\T{X} - \llbracket \T{X} \rrbracket_{\V{r}}\|_F + F_1(N)\|\T{\hat{X}} - \llbracket \hat{\T{X}}\rrbracket_{\mathbf{r}} \|_F  & \\
& \le F_2(N)\|\T{X} - \llbracket \T{X} \rrbracket_{\V{r}}\|_F + F_1(N)\|\T{\hat{X}}- \llbracket \T{X}\rrbracket_{\mathbf{r}} \|_F &
 \\
& \le F_2(N)\|\T{X} - \llbracket \T{X} \rrbracket_{\V{r}}\|_F + F_1(N)[\|\T{X}- \T{\hat{X}} \|_F +  \|\T{X}- \llbracket \T{X}\rrbracket_{\mathbf{r}} \|_F]\\
& \le (F_1(N)+F_2(N)+F1(N)F_2(N)) \|\T{X}- \llbracket \T{X}\rrbracket_{\mathbf{r}} \|_F.
\end{aligned}
\end{equation}
\end{proof}
