# Supplementary material for: Low-Rank Tucker Approximation of a Tensor From Streaming Data
Source: arXiv:1904.10951 source file (2021-04-30)
Supplement: Supplementary file 4 [file review_tensor_algorithmics.tex]

\section{Review of Tensor Arithmetic Operators}
\label{sec:review_tensor}
We review some basic tensor arithmetic operators.
Let $\T{X}$ be a tensor of shape $I_1\times I_2\times \dots \times I_N$.
Mode products commute: for $m \neq n \in [N]$,
\begin{equation}
\label{eq: tensor_product_mul_exchangable}
\T{X}\times_m \mathbf{A} \times_n \mathbf{B} =    \T{X}\times_n \mathbf{B} \times_m \mathbf{A}.
\end{equation}
Two mode products along the same mode simplify as
\begin{equation}
\label{eq: tensor_product_association}
\T{X}\times_n \mathbf{A} \times_n \mathbf{B} =    \T{X}\times_n (\mathbf{BA}). \nonumber
\end{equation}
The inner product for tensors matches the inner product for any mode-$n$ matricization:
\begin{equation}
\label{eq:F_norm_equivalent}
\langle \T{X}, \T{Y}\rangle = \langle \mathbf{X}^{(n)}, \mathbf{Y}^{(n)}\rangle = \rm{Tr}((\mathbf{X}^{(n)})^\top \mathbf{Y}^{(n)}).
\end{equation}
